# Supplementary material for: New ZrB$_2$ polymorphs: First-principles calculations
Source: arXiv:2005.12680 source file (2020-05-26)
Supplement: Supplementary file 1 [file SupplementaryInformationCombined.pdf]

*Supplementary information*

# New zirconium diboride polymorphs:

# First-principles calculations


*Marcin Maździarz, Tomasz Mościcki*

Institute of Fundamental Technological Research Polish Academy of Sciences,

Pawińskiego 5B, 02-106 Warsaw, Poland

E-mail: mmazdz@ippt.pan.pl

E-mail: tmosc@ippt.pan.pl

**CIF files:**

```
# ZrB2_191_LDA.cif

data_findsym-output
_audit_creation_method FINDSYM

_symmetry_space_group_name_H-M "P 6/m 2/m 2/m"
_symmetry_Int_Tables_number 191

_cell_length_a    3.13453
_cell_length_b    3.13453
_cell_length_c    3.47721
_cell_angle_alpha 90.00000
_cell_angle_beta  90.00000
_cell_angle_gamma 120.00000

loop_
_space_group_symop_id
_space_group_symop_operation_xyz
1 x,y,z
2 x-y,x,z
3 -y,x-y,z
4 -x,-y,z
5 -x+y,-x,z
6 y,-x+y,z
7 x-y,-y,-z
8 x,x-y,-z
9 y,x,-z
10 -x+y,y,-z
11 -x,-x+y,-z
```

12 -y,-x,-z

13 -x,-y,-z

14 -x+y,-x,-z

15 y,-x+y,-z

16 x,y,-z

17 x-y,x,-z

18 -y,x-y,-z

19 -x+y,y,z

20 -x,-x+y,z

21 -y,-x,z

22 x-y,-y,z

23 x,x-y,z

24 y,x,z

loop_

_atom_site_label

_atom_site_type_symbol

_atom_site_symmetry_multiplicity

_atom_site_Wyckoff_label

_atom_site_fract_x

_atom_site_fract_y

_atom_site_fract_z

_atom_site_occupancy

Zr1 Zr 1 a 0.00000 0.00000 0.00000 1.00000

B1 B 2 d 0.33333 0.66667 0.50000 1.00000

# ZrB2_191_PBE.cif

data_findsym-output

_audit_creation_method FINDSYM

_symmetry_space_group_name_H-M "P 6/m 2/m 2/m"

_symmetry_Int_Tables_number 191

_cell_length_a    3.17298

_cell_length_b    3.17298

_cell_length_c    3.52711

_cell_angle_alpha 90.00000

_cell_angle_beta  90.00000

_cell_angle_gamma 120.00000

loop_

_space_group_symop_id

_space_group_symop_operation_xyz

1 x,y,z

2 x-y,x,z

3 -y,x-y,z

4 -x,-y,z

5 -x+y,-x,z

6 y,-x+y,z

7 x-y,-y,-z

8 x,x-y,-z

9 y,x,-z

10 -x+y,y,-z

11 -x,-x+y,-z

12 -y,-x,-z

13 -x,-y,-z

14 -x+y,-x,-z

15 y,-x+y,-z

16 x,y,-z

17 x-y,x,-z

18 -y,x-y,-z

19 -x+y,y,z

20 -x,-x+y,z

21 -y,-x,z

22 x-y,-y,z

23 x,x-y,z

24 y,x,z

loop_

_atom_site_label

_atom_site_type_symbol

_atom_site_symmetry_multiplicity

_atom_site_Wyckoff_label

_atom_site_fract_x

_atom_site_fract_y

_atom_site_fract_z

_atom_site_occupancy

Zr1 Zr 1 a 0.00000 0.00000 0.00000 1.00000

B1 B 2 d 0.33333 0.66667 0.50000 1.00000

# ZrB2_191_PBEsol.cif

data_findsym-output

_audit_creation_method FINDSYM

_symmetry_space_group_name_H-M "P 6/m 2/m 2/m"

_symmetry_Int_Tables_number 191

_cell_length_a 3.15616

_cell_length_b 3.15616

_cell_length_c 3.49517

_cell_angle_alpha 90.00000

_cell_angle_beta 90.00000

_cell_angle_gamma 120.00000

loop_

_space_group_symop_id

_space_group_symop_operation_xyz

1 x,y,z

2 x-y,x,z

3 -y,x-y,z

4 -x,-y,z

5 -x+y,-x,z

6 y,-x+y,z

7 x-y,-y,-z

8 x,x-y,-z

9 y,x,-z

10 -x+y,y,-z

11 -x,-x+y,-z

12 -y,-x,-z

13 -x,-y,-z

14 -x+y,-x,-z

15 y,-x+y,-z

16 x,y,-z

17 x-y,x,-z

18 -y,x-y,-z

19 -x+y,y,z

20 -x,-x+y,z

21 -y,-x,z

22 x-y,-y,z

23 x,x-y,z

24 y,x,z

loop_

_atom_site_label

_atom_site_type_symbol

_atom_site_symmetry_multiplicity

_atom_site_Wyckoff_label

_atom_site_fract_x

_atom_site_fract_y

_atom_site_fract_z

_atom_site_occupancy

Zr1 Zr 1 a 0.00000 0.00000 0.00000 1.00000

B1 B 2 d 0.33333 0.66667 0.50000 1.00000

```
# ZrB2_194_LDA.cif

data_findsym-output
_audit_creation_method FINDSYM

_symmetry_space_group_name_H-M "P 63/m 2/m 2/c"
_symmetry_Int_Tables_number 194

_cell_length_a    3.02501
_cell_length_b    3.02501
_cell_length_c    8.51551
_cell_angle_alpha 90.00000
_cell_angle_beta  90.00000
_cell_angle_gamma 120.00000

loop_
_space_group_symop_id
_space_group_symop_operation_xyz
1 x,y,z
2 x-y,x,z+1/2
3 -y,x-y,z
4 -x,-y,z+1/2
5 -x+y,-x,z
6 y,-x+y,z+1/2
7 x-y,-y,-z
8 x,x-y,-z+1/2
9 y,x,-z
10 -x+y,y,-z+1/2
11 -x,-x+y,-z
12 -y,-x,-z+1/2
13 -x,-y,-z
```

14 -x+y,-x,-z+1/2

15 y,-x+y,-z

16 x,y,-z+1/2

17 x-y,x,-z

18 -y,x-y,-z+1/2

19 -x+y,y,z

20 -x,-x+y,z+1/2

21 -y,-x,z

22 x-y,-y,z+1/2

23 x,x-y,z

24 y,x,z+1/2

loop_

_atom_site_label

_atom_site_type_symbol

_atom_site_symmetry_multiplicity

_atom_site_Wyckoff_label

_atom_site_fract_x

_atom_site_fract_y

_atom_site_fract_z

_atom_site_occupancy

B1 B 4 f 0.33333 0.66667 0.02828 1.00000

Zr1 Zr 2 d 0.33333 0.66667 0.75000 1.00000

```
# ZrB2_194_PBE.cif

data_findsym-output
_audit_creation_method FINDSYM

_symmetry_space_group_name_H-M "P 63/m 2/m 2/c"
_symmetry_Int_Tables_number 194

_cell_length_a    3.07656
_cell_length_b    3.07656
_cell_length_c    8.62465
_cell_angle_alpha 90.00000
_cell_angle_beta  90.00000
_cell_angle_gamma 120.00000

loop_
_space_group_symop_id
_space_group_symop_operation_xyz
1 x,y,z
2 x-y,x,z+1/2
3 -y,x-y,z
4 -x,-y,z+1/2
5 -x+y,-x,z
6 y,-x+y,z+1/2
7 x-y,-y,-z
8 x,x-y,-z+1/2
9 y,x,-z
10 -x+y,y,-z+1/2
11 -x,-x+y,-z
12 -y,-x,-z+1/2
13 -x,-y,-z
```

14 -x+y,-x,-z+1/2

15 y,-x+y,-z

16 x,y,-z+1/2

17 x-y,x,-z

18 -y,x-y,-z+1/2

19 -x+y,y,z

20 -x,-x+y,z+1/2

21 -y,-x,z

22 x-y,-y,z+1/2

23 x,x-y,z

24 y,x,z+1/2

loop_

_atom_site_label

_atom_site_type_symbol

_atom_site_symmetry_multiplicity

_atom_site_Wyckoff_label

_atom_site_fract_x

_atom_site_fract_y

_atom_site_fract_z

_atom_site_occupancy

B1 B 4 f 0.33333 0.66667 0.02810 1.00000

Zr1 Zr 2 d 0.33333 0.66667 0.75000 1.00000

```
# ZrB2_194_PBEsol.cif

data_findsym-output
_audit_creation_method FINDSYM

_symmetry_space_group_name_H-M "P 63/m 2/m 2/c"
_symmetry_Int_Tables_number 194

_cell_length_a    3.05018
_cell_length_b    3.05018
_cell_length_c    8.56483
_cell_angle_alpha 90.00000
_cell_angle_beta  90.00000
_cell_angle_gamma 120.00000

loop_
_space_group_symop_id
_space_group_symop_operation_xyz
1 x,y,z
2 x-y,x,z+1/2
3 -y,x-y,z
4 -x,-y,z+1/2
5 -x+y,-x,z
6 y,-x+y,z+1/2
7 x-y,-y,-z
8 x,x-y,-z+1/2
9 y,x,-z
10 -x+y,y,-z+1/2
11 -x,-x+y,-z
12 -y,-x,-z+1/2
13 -x,-y,-z
```

14 -x+y,-x,-z+1/2

15 y,-x+y,-z

16 x,y,-z+1/2

17 x-y,x,-z

18 -y,x-y,-z+1/2

19 -x+y,y,z

20 -x,-x+y,z+1/2

21 -y,-x,z

22 x-y,-y,z+1/2

23 x,x-y,z

24 y,x,z+1/2

loop_

_atom_site_label

_atom_site_type_symbol

_atom_site_symmetry_multiplicity

_atom_site_Wyckoff_label

_atom_site_fract_x

_atom_site_fract_y

_atom_site_fract_z

_atom_site_occupancy

B1 B 4 f 0.33333 0.66667 0.02879 1.00000

Zr1 Zr 2 d 0.33333 0.66667 0.75000 1.00000

```
# ZrB2_59_LDA.cif

data_findsym-output
_audit_creation_method FINDSYM

_symmetry_space_group_name_H-M "P 21/m 21/m 2/n (origin choice 2)"
_symmetry_Int_Tables_number 59

_cell_length_a    3.05717
_cell_length_b    4.93098
_cell_length_c    4.54134
_cell_angle_alpha 90.00000
_cell_angle_beta  90.00000
_cell_angle_gamma 90.00000

loop_
_space_group_symop_id
_space_group_symop_operation_xyz
1 x,y,z
2 x+1/2,-y,-z
3 -x,y+1/2,-z
4 -x+1/2,-y+1/2,z
5 -x,-y,-z
6 -x+1/2,y,z
7 x,-y+1/2,z
8 x+1/2,y+1/2,-z

loop_
_atom_site_label
_atom_site_type_symbol
_atom_site_symmetry_multiplicity
```

```
_atom_site_Wyckoff_label
_atom_site_fract_x
_atom_site_fract_y
_atom_site_fract_z
_atom_site_occupancy
Zr1 Zr   2 b 0.25000 0.75000  0.38904  1.00000
B1  B    4 e 0.25000 -0.06056 -0.08705 1.00000
```

# ZrB2_59_PBE.cif

data_findsym-output

_audit_creation_method FINDSYM

_symmetry_space_group_name_H-M "P 21/m 21/m 2/n (origin choice 2)"

_symmetry_Int_Tables_number 59

_cell_length_a    3.10050

_cell_length_b    5.02883

_cell_length_c    4.60418

_cell_angle_alpha 90.00000

_cell_angle_beta  90.00000

_cell_angle_gamma 90.00000

loop_

_space_group_symop_id

_space_group_symop_operation_xyz

1 x,y,z

2 x+1/2,-y,-z

3 -x,y+1/2,-z

4 -x+1/2,-y+1/2,z

5 -x,-y,-z

6 -x+1/2,y,z

7 x,-y+1/2,z

8 x+1/2,y+1/2,-z

loop_

_atom_site_label

_atom_site_type_symbol

_atom_site_symmetry_multiplicity

_atom_site_Wyckoff_label

_atom_site_fract_x

_atom_site_fract_y

_atom_site_fract_z

_atom_site_occupancy

Zr1 Zr   2 b 0.25000 0.75000  0.38562  1.00000

B1  B    4 e 0.25000 -0.06195 -0.08857 1.00000

```
# ZrB2_59_PBEsol.cif

data_findsym-output
_audit_creation_method FINDSYM

_symmetry_space_group_name_H-M "P 21/m 21/m 2/n (origin choice 2)"
_symmetry_Int_Tables_number 59

_cell_length_a    3.07143
_cell_length_b    4.98134
_cell_length_c    4.57772
_cell_angle_alpha 90.00000
_cell_angle_beta  90.00000
_cell_angle_gamma 90.00000

loop_
_space_group_symop_id
_space_group_symop_operation_xyz
1 x,y,z
2 x+1/2,-y,-z
3 -x,y+1/2,-z
4 -x+1/2,-y+1/2,z
5 -x,-y,-z
6 -x+1/2,y,z
7 x,-y+1/2,z
8 x+1/2,y+1/2,-z

loop_
_atom_site_label
_atom_site_type_symbol
_atom_site_symmetry_multiplicity
```

_atom_site_Wyckoff_label

_atom_site_fract_x

_atom_site_fract_y

_atom_site_fract_z

_atom_site_occupancy

Zr1 Zr 2 b 0.25000 0.75000 0.38692 1.00000

B1 B 4 e 0.25000 -0.06193 -0.08932 1.00000

**Phonons:**

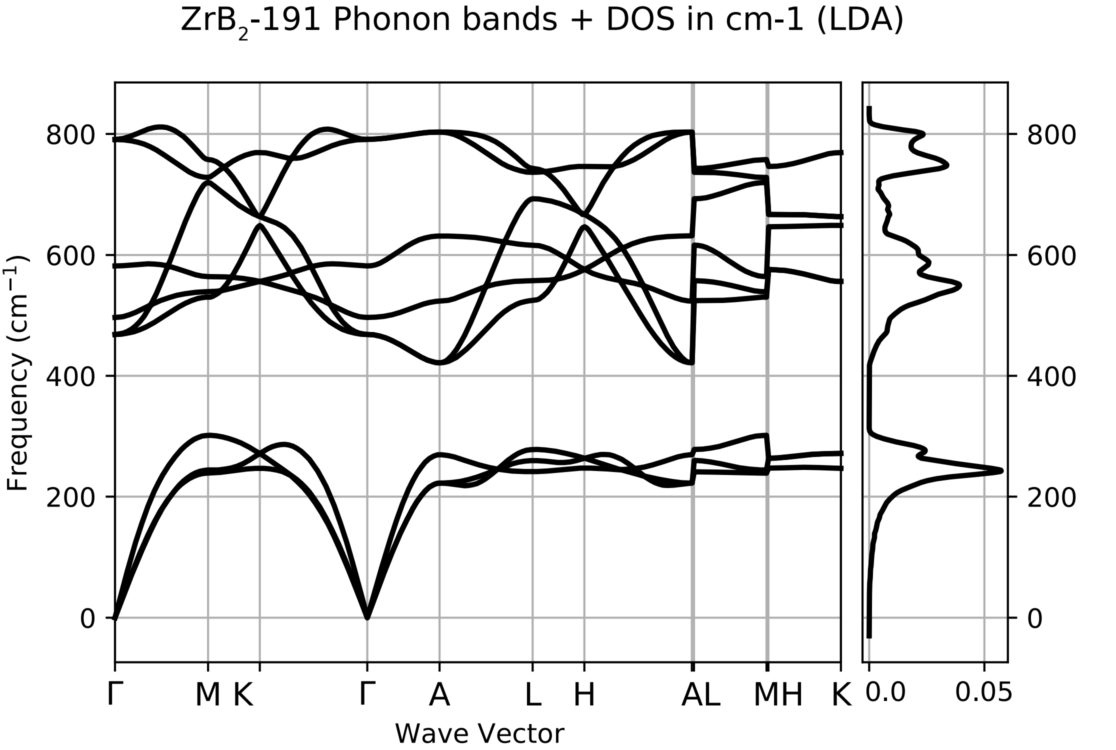

ZrB$_2$-191 Phonon bands + DOS in cm-1 (LDA)
Frequency (cm$^{-1}$)
800
600
400
200
0
Γ
M
K
Γ
A
L
H
AL
MH
K
Wave Vector
0.0
0.05

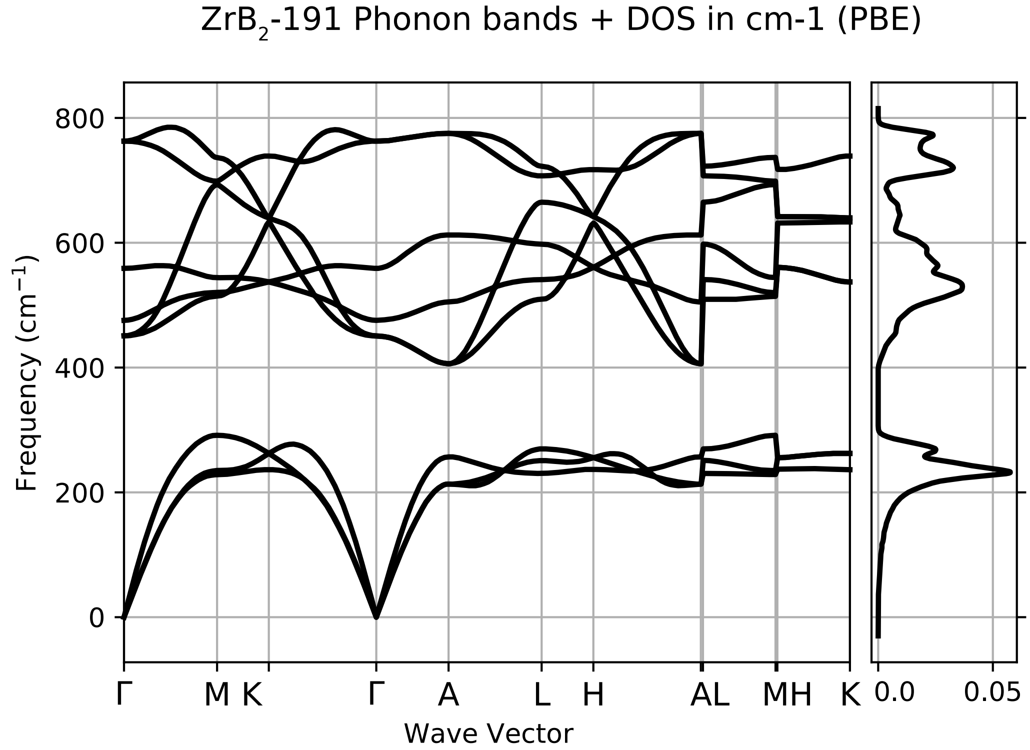

ZrB$_2$-191 Phonon bands + DOS in cm-1 (PBE)
Frequency (cm$^{-1}$)
800
600
400
200
0
Γ
M K
Γ
A
L
H
AL
MH
K
Wave Vector
0.0
0.05

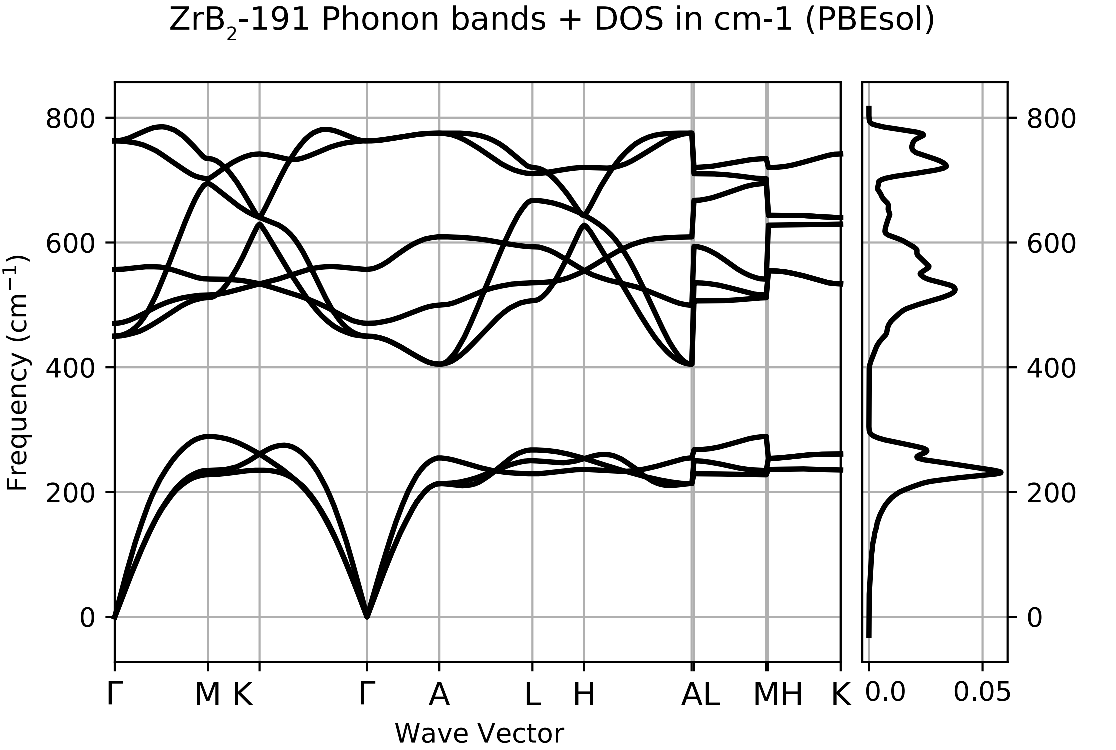

ZrB$_2$-191 Phonon bands + DOS in cm-1 (PBEsol)
Frequency (cm$^{-1}$)
800
600
400
200
0
Γ
M
K
Γ
A
L
H
AL
MH
K
Wave Vector
0.0
0.05
800
600
400
200
0

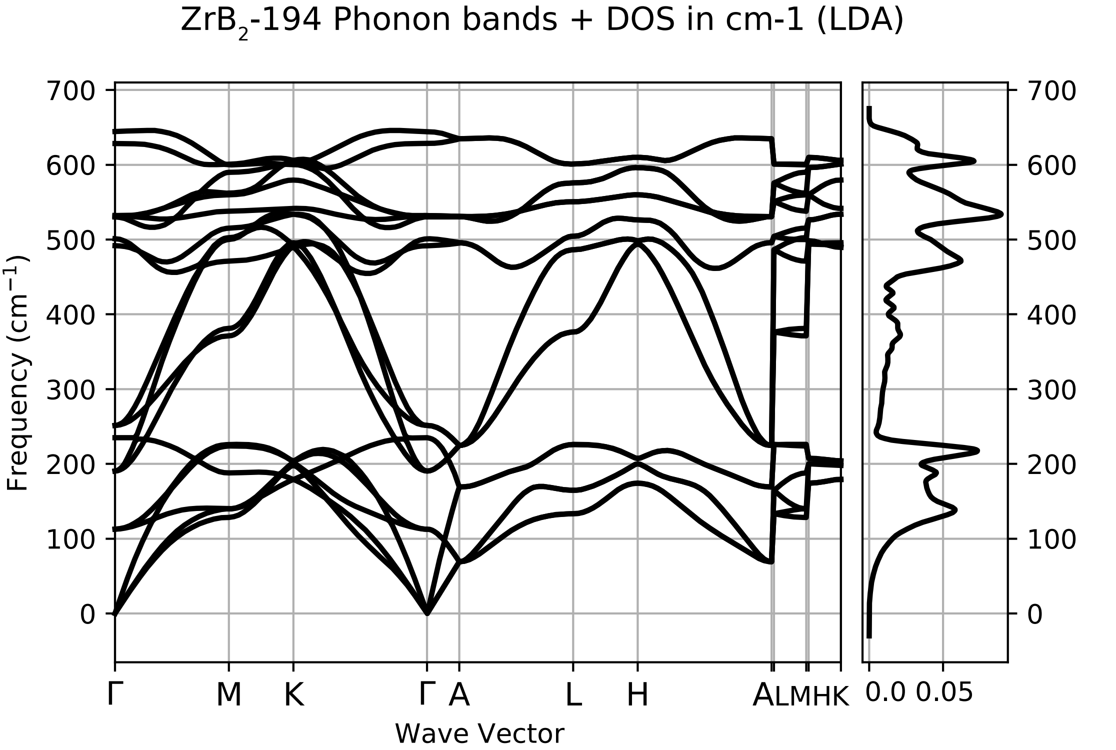

ZrB2-194 Phonon bands + DOS in cm-1 (LDA)
Frequency (cm−1)
Wave Vector
700
600
500
400
300
200
100
0
Γ
M
K
Γ
A
L
H
ALMHK
0.0
0.05

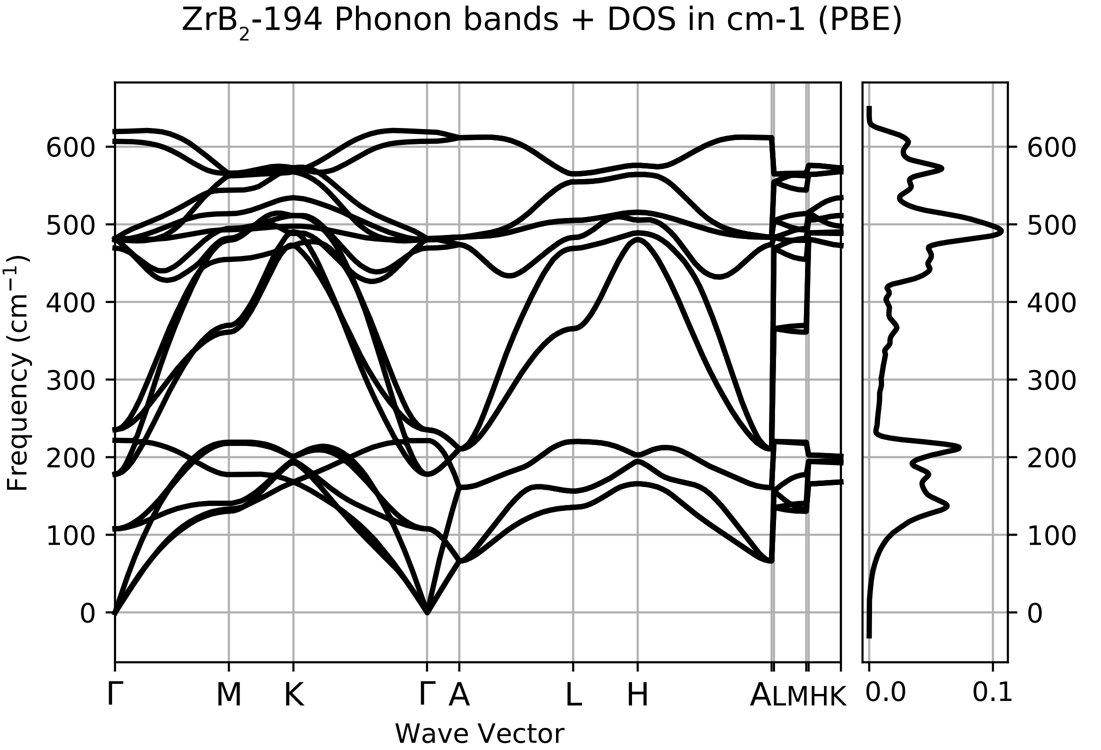

ZrB$_2$-194 Phonon bands + DOS in cm-1 (PBE)
Frequency (cm$^{-1}$)
Wave Vector
Γ
M
K
Γ
A
L
H
ALMHK
0
100
200
300
400
500
600
0.0
0.1

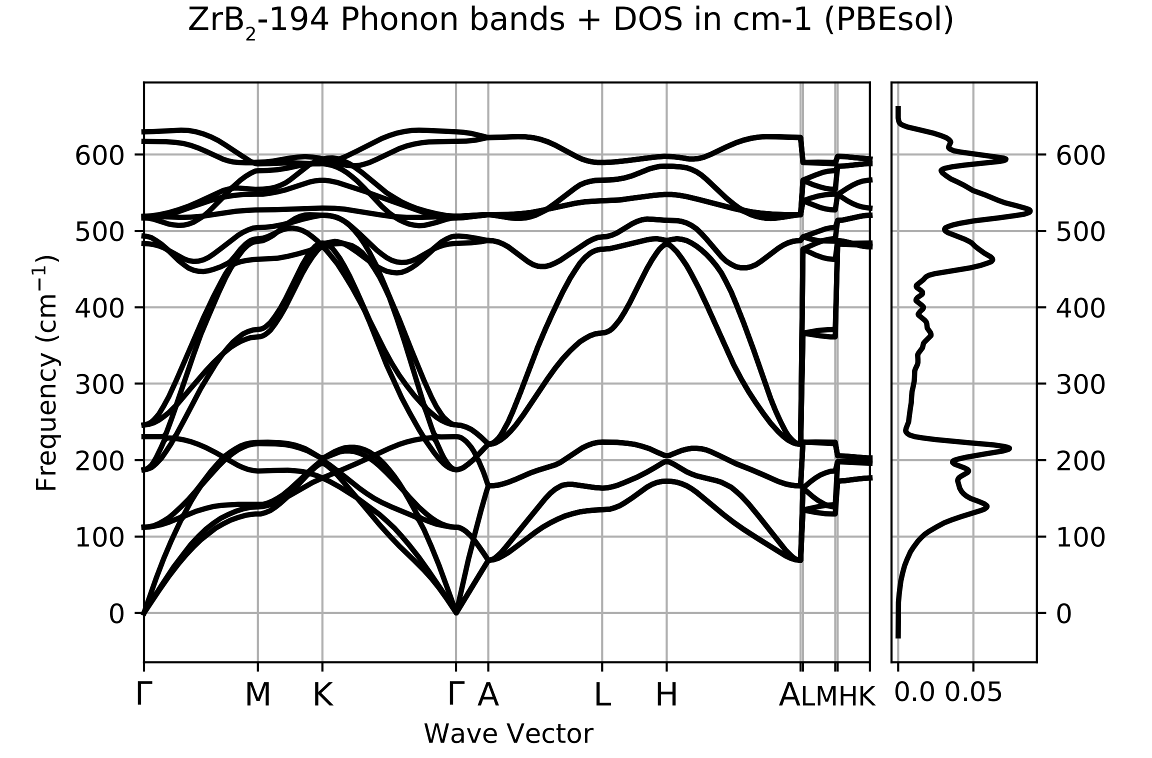
ZrB2-194 Phonon bands + DOS in cm-1 (PBEsol)
Frequency (cm−1)
600
500
400
300
200
100
0
Γ
M
K
Γ
A
L
H
A
L
M
H
K
Wave Vector
0.0
0.05

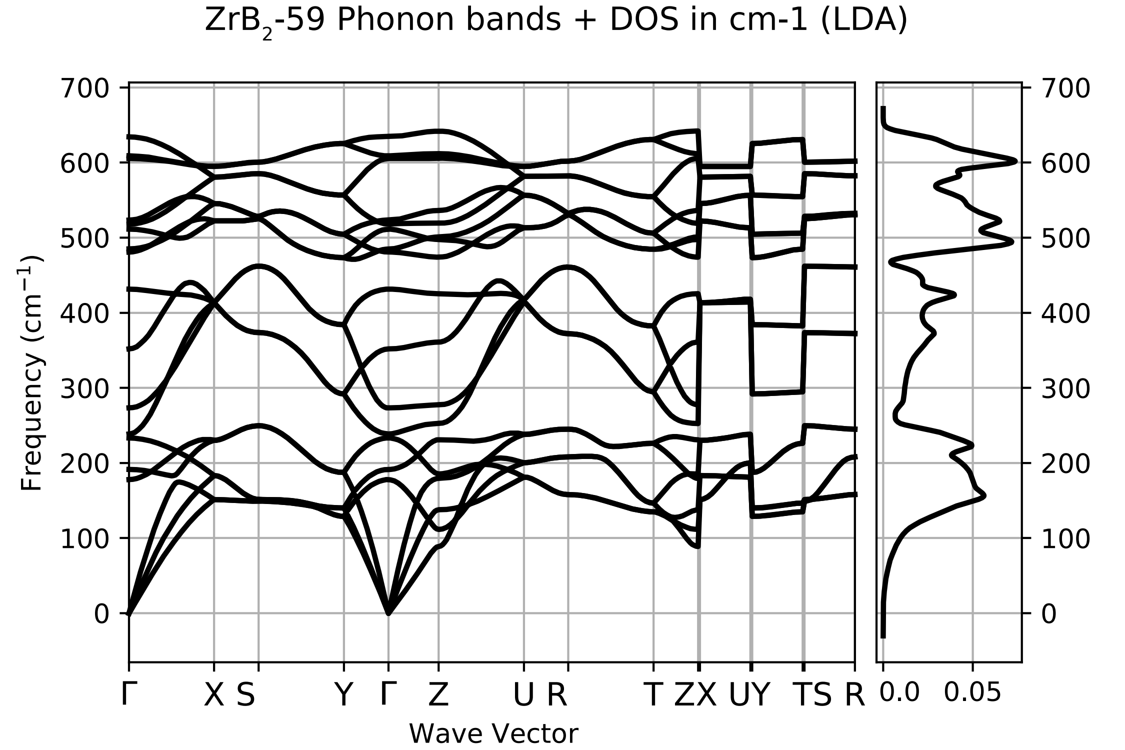

ZrB2-59 Phonon bands + DOS in cm-1 (LDA)
Frequency (cm−1)
700
600
500
400
300
200
100
0
Γ
X S
Y Γ
Z
U R
T ZX UY
TS R
Wave Vector
0.0
0.05

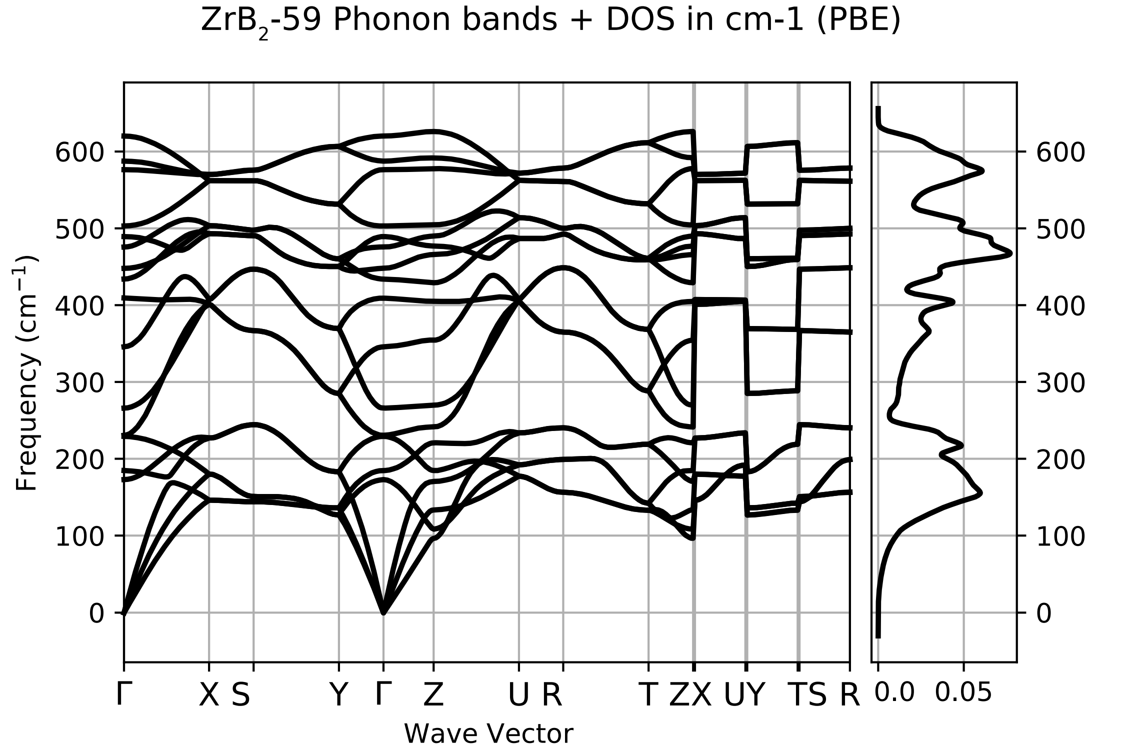
ZrB2-59 Phonon bands + DOS in cm-1 (PBE)
Frequency (cm−1)
600
500
400
300
200
100
0
Γ
X S
Y Γ
Z
U R
T ZX UY
TS R
Wave Vector
0.0
0.05

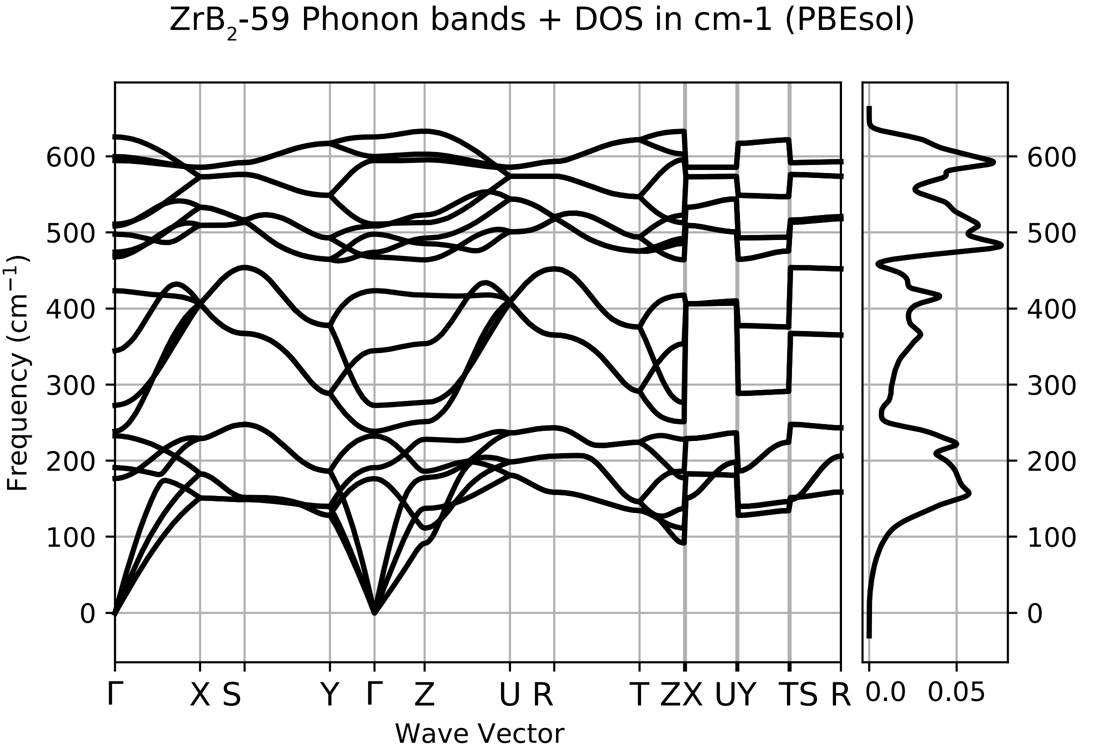
ZrB2-59 Phonon bands + DOS in cm-1 (PBEsol)
Frequency (cm−1)
Wave Vector
Γ
X S
Y
Γ
Z
U R
T ZX UY
TS R
0
100
200
300
400
500
600
0.0
0.05
